# Supplementary material for: Cost-Effective Algorithms for Average-Case Interactive Graph Search
Source: arXiv:2201.07944 source file (2022-01-20)
Supplement: Supplementary file 1 [file Appendix.tex]

\section{Missing Proofs}
For ease of reference, we first restate all the lemmas and theorems and then provide the formal proofs.

\subsection{Proof of Lemma~\theIGStosearchinposet}
\begin{lemma}\label{the:np_hardness_for_IGS_appendix}%[Lemma~\theIGStosearchinposet]
AIGS is NP-hard. In fact, there cannot be any $o(\log n)$-approximate algorithm for AIGS unless $\mathrm{NP} \subseteq \mathrm{DTIME}(n^{O(\log\log n)})$.
\end{lemma}
To prove Lemma~\ref{the:np_hardness_for_IGS_appendix} (i.e.,~Lemma~\theIGStosearchinposet), we begin by showing that the IGS problem is equivalent to the search in poset problem~\cite{daskalakis2011sorting}. We first formally define the partially ordered set.

\begin{definition}[Partially Ordered Set]
A partially ordered set is a pair $(V,\le_R)$, where $V$ is a set of objects and $\le_R$ is a partially ordered relation which satisfies the following properties:
\begin{itemize}
    \item Reflexivity: $a \le_R a$.
    \item Antisymmetry: if $a \le_R b$ and $b \le_R a$, then $a=b$. \item Transitivity: if $a \le_R b$ and $b \le_R c$, then $a \le_R c$. 
\end{itemize}
\end{definition}

Reflexivity shows that every object is related to itself. Antisymmetry indicates that for any two distinct objects, they cannot relate to each other. Transitivity reflects that the relation is transitive.

\begin{definition}[Search in Poset]
Given an (unknown) target object $z$ in a poset $(V,\le_R)$, the search problem aims to locate the target objects by queries. To search the target object, each query on object $x\in V$ will return a boolean result:
\begin{itemize}
	\item \textit{yes}, if the target object is related to $x$.
	\item \textit{no}, otherwise.
\end{itemize}
\end{definition}
We make a connection between the IGS problem and the search problem in poset.
\begin{lemma}\label{the:IGS_to_searchinposet_appendix}
	The IGS problem is equivalent to the search problem in a poset.
\end{lemma}
\begin{proof}%[Proof of Lemma~\ref{the:IGS_to_searchinposet_appendix}]
	The reachability of IGS satisfies the following properties.
	\begin{itemize}
		\item Reflexivity: Each node can reach itself.
		\item Antisymmetry: For two nodes $u,v$, if $u$ can reach $v$ and $v$ can reach $u$, then $u$ should equal to $v$.
		\item Transitivity: For three nodes $u,v,w$, if $u$ can reach $v$ and $v$ can reach $w$, then $u$ can reach $w$ by taking $v$ as a relay node.
	\end{itemize}
	Hence, the reachability relation in the IGS problem is a partially ordered relation. Moreover, given a target node $z\in V$, the query on node $q\in V$ will get a \textit{yes} answer if and only if $z$ is reachable from $q$, which satisfies query in a poset. Therefore, the IGS problem is a search problem in a poset.
	
	On the other hand, given a poset, we can construct a DAG hierarchy as follows. For any two distinct objects $a$ and $b$ in the poset, if $a\leq_R b$ and there does not exist any $c\in V\setminus\{a,b\}$ such that $a\leq_R c$ and $ c\leq_R b$, i.e.,~$a$ is directly related to $b$, then $a$ is the child of $b$ in the hierarchy. It is easy to verify that the constructed hierarchy is a DAG and for two objects $a$ and $b$ satisfying $a\leq_R b$, it must hold that $a$ is reachable from $b$ in the hierarchy. This implies that searching a poset can be represented by an IGS problem.
\end{proof}

Now we are ready to prove Lemma~\ref{the:np_hardness_for_IGS_appendix} (i.e.,~Lemma~\theIGStosearchinposet).
\begin{proof}[Proof of Lemma~\ref{the:np_hardness_for_IGS_appendix}]
    \citet{cicalese2011complexity} proved that deriving the optimal solution for the average-case poset search is NP-hard even if the poset has a tree structure (i.e.,~the input hierarchy of AIGS is a tree). Moreover, \citet{cicalese2011complexity} pointed out that for the problem of minimizing the weighted average number of queries to identify an initially unknown object for general posets, there cannot be any $o(\log n)$-approximate algorithm unless $\mathrm{NP} \subseteq \mathrm{DTIME}(n^{O(\log\log n)})$, where $n$ is the number of nodes. Combining with Lemma~\ref{the:IGS_to_searchinposet_appendix} completes the proof.
\end{proof}

\subsection{Proof of Theorem~\thmroundgreedy}
\begin{theorem}\label{thm:round-greedy_appendix}%[Theorem~\thmroundgreedy]
The rounded greedy algorithm provides an approximation ratio of $2(1+3\ln n)$ for AIGS.
\end{theorem}
To prove Theorem~\ref{thm:round-greedy_appendix} (i.e., Theorem~\thmroundgreedy), we make the connection between our AIGS problem and the decision tree problem~\cite{garey1972optimal,chakaravarthy2007decision}. In particular, a target node of AIGS corresponds to an object of decision tree while a query node of AIGS corresponds to a test of decision tree (i.e., whether the target node is reachable from the query node). Hence, we revisit the AIGS problem from the view of the decision tree problem.

Devising a query policy for the AIGS problem can be modeled as a \textit{decision tree} construction problem. In particular, as the answer is a boolean, i.e.,~\textit{yes} or \textit{no}, a binary decision tree is considered in practice. In the following, we show how to construct a binary decision tree according to the search strategy of AIGS and calculate the cost based on the constructed decision tree.

\begin{definition}[Decision Tree for AIGS]
	We model the query policy of AIGS as a decision tree, where each internal node represents a question (i.e.,~the query node) and each leaf node represents a search result (i.e.,~the target node). Starting from the root of a decision tree, the algorithm asks questions following the below rules.
	\begin{itemize}
		\item If the answer is \textit{yes}, i.e.,~the target node is reachable from the query node, it goes to the left child.
		\item Otherwise, if the answer is \textit{no}, it goes to the right child.
	\end{itemize}
	The above process stops at a leaf node, which will be returned as the search result.
\end{definition}

According to the above definition, it is trivial to see that given any DAG $G$, the size of its decision tree $D$ is at most twice the size of $G$, since every node of $G$ appears as a leaf node of $D$ whereas at most all nodes of $G$ serve as internal nodes of $D$. Furthermore, it is easy to observe that the number of questions asked for identifying a target node equals to the depth of the corresponding leaf node in $D$, i.e.,~the length of its path from the root in $D$. Meanwhile, the weight of each leaf node $v$ equals to the probability $p(v)$ of the node $v$ being the target node. Hence, we formally define the cost of a query policy leveraging the notion of decision tree. 
\begin{definition}[Cost of Query Policy]\label{def:cost1}
	Given a query policy for the AIGS problem, let $D$ be the decision tree constructed according to the policy. Denote by $L(D)$ the set of all leaf nodes in $D$, and by $h(v)$ the depth of every leaf node $v\in L(D)$. Then, the cost of $D$, i.e.,~the expected cost of the query policy, is given by
	\begin{equation}\label{eq:cost1}
	cost(D)=\sum_{v \in L(D)}p(v)h(v).
	\end{equation}
\end{definition}
Now we are ready to prove Theorem~\ref{thm:round-greedy_appendix} (i.e., Theorem~\thmroundgreedy).
\begin{proof}[Proof of Theorem~\ref{thm:round-greedy_appendix}]
    Our above analysis shows that AIGS can be transferred to a special case of average-case binary decision tree. In addition, \citet{chakaravarthy2007decision} proved that the rounded greedy policy achieves an approximation ratio of $2(1+3\ln n)$ for average-case binary decision tree. Therefore, the theorem is proved.
\end{proof}

% \begin{figure*}[!hbpt]
% 	\centering
% 	\subfloat[An Input Hierarchy]{\includegraphics[width=0.25\textwidth]{figs/IGS-GraphExample.pdf}\label{fig:IGS-GraphExample}}\hfil
% 	\subfloat[Decision Tree]{\includegraphics[width=0.5\textwidth]{figs/IGS-DT_Example.pdf}\label{fig:IGS-DTExample}}
% 	\caption{Decision tree for the query policy of AIGS.}\label{fig:IGS-DT}
% \end{figure*}
% \begin{example}
% \figurename~\ref{fig:IGS-DT} gives the graph representation of the hierarchy given in \figurename~\figExampleCategoryIdentification. Suppose that the nodes have equal weights, i.e.,~$p(v)=1/7$ for every $v\in V$. Figure~\figIGSDTExample shows the decision tree of a (greedy) policy. Assume that node $5$ is the target node. Then, the algorithm will sequentially query on nodes $3$, $4$ and $5$ with answers of \textit{no}, \textit{no} and \textit{yes}, respectively, so that the target node is figured out with no ambiguity. Moreover, the expected cost of this policy is $\frac{1}{7}\times(2\times 2+ 3\times 3 + 2\times 4)=3$.
% \end{example}
\subsection{Proof of Theorem~\thmgreedytree}
\begin{theorem}\label{the:IGS_tree_approximation_ratio_appendix}%[Theorem~\thmgreedytree]
    If the input hierarchy is a tree, the greedy policy provides an approximation ratio of $\frac{1+\sqrt{5}}{2}$ for AIGS.
\end{theorem}
\begin{proof}
    Let $\widetilde{D}$ be the decision tree constructed by greedy policy and $D^\ast$ be the optimal decision tree, with respect to the cost function defined in \eqref{eq:cost1}. For such a tree-like poset, \citet{cicalese2014improved} proved that the cost of $\widetilde{D}$ satisfies
    \begin{equation}
    cost(\widetilde{D}) \le \frac{1+\sqrt{5}}{2}\cdot cost(D^\ast).
    \end{equation}
    Furthermore, according to Lemma~\ref{the:IGS_to_searchinposet_appendix}, we know that $cost(\widetilde{D})$ is exactly the expected number of questions asked by the greedy policy for AIGS. Putting it together completes the proof.
\end{proof} 

\subsection{Proof of Theorem~\thmgreedyequalprob}
\begin{theorem}\label{the:IGS_equal_prob_approximation_ratio_appendix}%[Theorem~\thmgreedyequalprob]
	If every node has an equal probability to be the target node, i.e., $p(v)=1/n$ for every $v\in n$, the greedy policy provides an approximation ratio of $O\left(\frac{\log n}{\log \log n}\right)$ for AIGS.
\end{theorem}
\begin{proof}
    \citet{li2020tight} showed that for any instance of the decision tree problem on $n$ objects with equal probability to be the target, the greedy decision tree $\widetilde{D}$ and the optimal decision tree $D^\ast$ satisfy
    \begin{equation*}
    cost(\widetilde{D}) \le \frac{6 \log n}{\log cost(D^\ast)}\cdot cost(D^\ast).
    \end{equation*}
    Moreover, for any binary tree with $n$ leaf nodes, it is trivial to verify that the total depth of all leaf nodes is minimized on the complete binary tree, which is at least $n\log_2 n$. This implies the optimal solution has a cost of at least $\log_2 n$. As a result, the greedy policy returns a $O\left(\frac{\log n}{\log \log n}\right)$-approximate solution for AIGS when every node has an equal probability to be the target node. Hence, the theorem is proved.
\end{proof}

\subsection{Proof of Theorem~\thmMiddlePointonHeavyPath}
\begin{theorem}\label{thm:Middle_Point_on_Heavy_Path_appendix}%[Theorem~\thmMiddlePointonHeavyPath]
Given a tree $T$, let $H(T,r)$ be the weighted heavy path containing the root $r$ of $T$, with respect to the node probability. Then, the node $u\in H(T,r)$ that minimizes $\abs{2\cdot p(T_u)-p(T)}$ is the middle point of $T$, where $T_u$ denotes the subtree of $T$ rooted at $u$.
\end{theorem}
\begin{proof}
	Consider any internal node $u\in T$, let $v$ be the child of $u$ such that the edge $(u,v)$ is heavy and $x$ be any other child of $u$. Clearly, it holds that $p(T_u)\geq 2p(T_x)$, since $p(T_v)\geq p(T_x)$ and $p(T_u)\geq p(T_v)+p(T_x)+p(u)$. Thus,
	\begin{equation*}
		\abs{2p(T_x)-p(T)}=p(T)-2p(T_x).
	\end{equation*}
	Moreover, for any descendant $y$ of $x$, we have $p(T_x)\geq p(T_y)$, which indicates that
	\begin{equation*}
		\abs{2p(T_y)-p(T)}=p(T)-2p(T_y)\geq p(T)-2p(T_x).
	\end{equation*}
	
	Now, we consider the node $v$. There are two cases: (i) $p(T)\geq 2p(T_v)$ and (ii) $p(T)< 2p(T_v)$. For case (i), obviously,
	\begin{equation*}
		\abs{2p(T_v)-p(T)}=p(T)-2p(T_v)\leq p(T)-2p(T_x).
	\end{equation*}
	For case (ii), as $p(T_v)+p(T_x)\leq p(T)$, it also holds that
	\begin{equation*}
	\abs{2p(T_v)-p(T)}=2p(T_v)-p(T)\leq p(T)-2p(T_x).
	\end{equation*}
	
	Putting it together, we have
	\begin{equation*}
		\abs{2p(T_v)-p(T)}\leq \abs{2p(T_x)-p(T)}\leq \abs{2p(T_y)-p(T)}.
	\end{equation*}
	This implies that $v$ dominates all other children of $u$ as well as all their descendants. Hence, starting with $u=r$, we just keep the subtree rooted at the child $v$ of $u$ such that the edge $(u,v)$ is heavy, and meanwhile remove all subtrees rooted at the other children of $u$, since all nodes in latter are dominated by $v$. We then set $u=v$ and repeat the process until $v$ is a leaf node. This procedure actually generates the weighted heavy path $H(T,r)$ containing the root $r$ of $T$. Therefore, by definition, the node $u\in H(T,r)$ that minimizes $\abs{2\cdot p(T_u)-p(T)}$ is the middle point of $T$.
\end{proof}

\section{Naive Instantiation of Greedy}\label{sec:algorithm-appendix}
Algorithm~\ref{alg:BIGS_naive} gives the pseudo-code for a naive implementation of the greedy policy, referred to as \greedyN. To find the middle point in each round of query, the algorithm enumerates all candidate nodes and computes the total probability of all nodes reachable from every node independently (Lines~\ref{algline:q_start}--\ref{algline:q_end}). In particular, the total probability of the subgraph rooted at $v$ is calculated via a subroutine \getp given by Algorithm~\ref{alg:get_subgraph_weight} (Line~\ref{algline:q_prob}). Given a graph $G$ and a query node $v$, the \getp algorithm performs a breadth first search (BFS) that starts from $v$, which can introduce heavy computational overhead. A similar BFS will be performed for the graph update after finding the middle point (Lines~\ref{algline:update-Gq} and \ref{algline:update-not-Gq}).

\begin{algorithm}[!tbp]
	\caption{$\greedyN(G)$}
	\label{alg:BIGS_naive}
	\KwIn{an input DAG $G$}
	\KwOut{the target node}
	$sum\_prob \gets 1$\;
	\While{$\abs{G}>1$}{
		$min\_prob \gets +\infty$\;\label{algline:q_start}
		\ForEach{node $v \in G$}{
			$reach\_prob \gets \getp(G,v)$\;\label{algline:q_prob}
			\If{$\abs{2\cdot reach\_prob-{sum\_prob}} < min\_prob$}{
				$q \gets v$\;
				$q\_prob \gets reach\_prob$\;
				$min\_prob\gets \abs{2\cdot reach\_prob-{sum\_prob}}$\;\label{algline:q_end}
			}
		}
		\uIf{$reach(q)=yes$}{
			$G\gets G_q$\;\label{algline:update-Gq}
			$sum\_prob \gets q\_prob$\;
		}
		\Else{
			$G\gets G\setminus G_q$\;\label{algline:update-not-Gq}
			$sum\_prob \gets sum\_prob-q\_prob$\;
		}
	}
	\Return{the only node in $G$\;}
\end{algorithm}

\begin{algorithm}[!tbp]
    \caption{$\getp(G,v)$}
    \label{alg:get_subgraph_weight}
    \KwIn{a DAG $G$ and a node $v$}
    \KwOut{the total probability of all $v$'s reachable nodes in $G$}
    $prob \gets 0$\;
    initialize a queue $S$ and insert the node $v$ into $S$\;
    mark every node in $G$ as \textit{unvisited}\;
    \While{$S$ is not empty}{
        push out a node from $S$ as $u$\;
        \ForEach{child $v$ of $u$}{
            \If{$v$ is not visited}{
                $prob \gets prob+p(v)$\;
                insert $v$ into $S$\;
                mark $v$ as \textit{visited}\;
            }
        }
    }
    \Return{$prob$\;}
\end{algorithm}

\section{Additional Explanations of Experiments}
% In this section, we provide more detail of the experiment section.
%We further introduce the statistic and the competing algorithms.

\subsection{Datasets}
\begin{itemize}[topsep=2mm, partopsep=0pt, itemsep=1mm, leftmargin=18pt]
	\item Amazon~\cite{he2016ups}. This is a  dataset including the product hierarchy at Amazon with a tree structure. This dataset contains information of products sold at Amazon, like reviews and product metadata. Specifically, the record has a field named \textit{categories}, and we can consider this field as a path starting from the root of the hierarchy to this product category. By combining these paths together, we can get a tree hierarchy with 29,240 nodes.
	\item ImageNet~\cite{deng2009imagenet}. This is a large-scale hierarchical image dataset using the structure of WordNet~\cite{miller1998wordnet}. Each category is represented as a tag called as \textit{synset} in the XML file (\url{https://www.imagenet.org/api/xml/structure_released.xml}), and the subcategory is given inside each tag explicitly. The attribute \textit{wnid} of each tag assigns an unique id to each category. We note that the category with $\textit{wnid}=\text{``fa11misc''}$ contains miscellaneous images that do not conform to WordNet. We extract all categories except the one with $\textit{wnid}=\text{``fa11misc''}$ and get a DAG with 27,714 nodes.
\end{itemize}

% \begin{table*}[!tbp]
% 	\caption{Comparison with previous works with yes-or-no query}
% 	\label{tab:compare_works}
% 	\centering
% 	\vspace{-1mm}
% 	\begin{tabular}{cccccc}
% 		\toprule
% 		\textbf{Method} & \textbf{Interactive} & \textbf{Graph Type} & \textbf{\# Queries (Worst Case)} & \textbf{\# Queries (Average Case)} &\textbf{Time (Each Query)}\\
% 		\midrule
% % 		HGS-T~\cite{parameswaran2011human} & No & Tree & n-1 & / & / \\
% % 		HGS-G~\cite{parameswaran2011human} & No & DAG & n-1 & / & / \\
% 		TopDown~\cite{Tao:IGS} & Yes & DAG & n-1 & / & $O(1)$\\
% 		WIGS~\cite{Tao:IGS} & Yes & DAG & $\left\lceil\log _{2} h\right\rceil\left(1+\left\lfloor\log _{2} n\right\rfloor\right)+(d-1) \cdot\left\lceil\log _{d} n\right\rceil$ & / & $O(1)$\\
% 		Greedy-T & Yes & Tree & / & $\le (\sqrt{5}+1)/2*OPT$ & $O(hd)$\\
% 		Greedy-D & Yes & DAG & / & $\le 2(\ln 3+1)*OPT$ & $O(m)$\\
% 		\bottomrule
% 	\end{tabular}
% 	\vspace{-1mm}
% \end{table*}

% \begin{table*}[!tbp]
% 	\caption{Comparison with previous works with multiple-choice query}
% 	\label{tab:compare_works_mc}
% 	\centering
% 	\vspace{-1mm}
% 	\begin{tabular}{cccccc}
% 		\toprule
% 		\textbf{Method} & \textbf{Interactive} & \textbf{Graph Type} & \textbf{\# Queries (Worst Case)} & \textbf{\# Queries (Average Case)} &\textbf{Time (Each Query)}\\
% 		\midrule
% 		MIGS~\cite{li2020efficient} & Yes & Tree & / & $\le 2*OPT$ & $O(n)$\\
% 		\bottomrule
% 	\end{tabular}
% 	\vspace{-1mm}
% \end{table*}

\subsection{Competing Algorithms}

\spara{\textbf{\topdown}~\cite{Tao:IGS}}
This is a naive way to solve the IGS problem. The \topdown method will ask questions from the root of the hierarchy. Note that the performance of the \topdown method is sensitive to the order of child nodes. All the performance of \topdown in this section is averaged from 20 runs by randomly permuting the order of child nodes before each run.

\spara{\textbf{\igs}~\cite{Tao:IGS}}
This is the state-of-the-art algorithm for IGS problem. \citet{Tao:IGS} proposed the \textsf{ordered-interleave} and \textsf{DFS-interleave} algorithms for the worst-case IGS problem given the input hierarchy is a tree and DAG, respectively. For convenience, we will abuse the name \igs to represent the two algorithms.

\spara{\textbf{\migs}~\cite{li2020efficient}}
This is an algorithm leveraging the multiple-choice query to solve the IGS problem. It is unfair to compare our algorithm with their algorithm directly, since the multiple-choice query proposed by their algorithm will give much more information. We notice that the crowd will read the multiple choices one by one and consider each choice is correct or not during the categorization process. The effort to judge a choice is similar to the effort to answer an yes-or-no query. Hence, we will consider the number of choices read by the crowd as the cost of their algorithm. Since the MIGS is also sensitive to the order of child nodes, we evaluate its performance from the average cost of 20 runs with random permutation on the order of child nodes as well. The algorithm proposed in~\cite{li2020efficient} is designed. We adapt the original algorithm to DAG with the same criterion. In the adapted algorithm, we will choose the node which makes the heaviest subgraph as light as possible in each round.

\subsection{Additional Experimental Results}
For the AIGS problem where the probability of each node is identical,  we study the average number of questions asked for identifying target nodes placed at different depths. For each depth value $d$, we calculated the average number of queries for locating all nodes of depth $d$. We also use the candidate set size (CSS) to measure the progressiveness. Specifically, CSS is the number of nodes that are potential to be the target node, which decreases as long as the algorithm executes. The target node will be returned by the algorithm when CSS drops to $1$.

\figurename~\ref{fig:uniformIGS_performance_vs_layers} shows the experiment result for the comparison between our \greedy algorithm and the state-of-the-art \igs algorithm. We observe from \figurename~\ref{fig:uniformIGS_performance_vs_layers_amazon} that on the Amazon dataset, our algorithm almost always asks fewer questions than \igs for all depths. We also find that the number of queries generally decreases along with the node depth. The reason is that when a target node is close to the root, each query by \greedy usually eliminates a subgraph rooted at a deeper level of the input hierarchy, which requires relatively more queries to locate the target node. On the ImageNet dataset, \figurename~\ref{fig:uniformIGS_performance_vs_layers_imagenet} shows a similar trend except the depth $0$. The reason is explained as follows. We node that \igs first performs a binary search on the heavy path to find the last node $u$ with $reach(u) = yes$ and then finds the leftmost child $v$ of $u$ with $reach(v) = yes$. Thus, when the root $r$ is the target node, \igs will quickly find $u=r$ and query on every child of $r$. By extracting the datasets, we find that the out-degree of the root is $84$ on Amazon, whereas the value is $8$ on ImageNet. As a result, \igs asks around $90$ and $10$ questions on the two datasets, respectively.
\begin{figure}[!tbp]
	\centering
	\subfloat[Amazon]{\includegraphics[width=0.3\textwidth]{figs/IGS_VS_BIGS_Tree.pdf}\label{fig:uniformIGS_performance_vs_layers_amazon}}\hfil
	\subfloat[ImageNet]{\includegraphics[width=0.31\textwidth]{figs/IGS_VS_BIGS_DAG.pdf}\label{fig:uniformIGS_performance_vs_layers_imagenet}}
% 	\vspace{-0.1in}
	\caption{Cost vs.\ node depth under equal probability setting.}
	\label{fig:uniformIGS_performance_vs_layers}
% 	\vspace{-0.1in}
\end{figure}

\figurename~\ref{fig:uniformIGS_Progressiveness} shows the average CSS against the number of queries to demonstrate the progressiveness of our approach. To get the average CSS, we record all the candidate set sizes after each query during the search process for all possible target nodes. After that, we will have $n$ arrays denoted as $\mathrm{CCS}_u$, where $\mathrm{CCS}_u[i]$ equals to the number of nodes in the candidate set after asking $i$ questions given the target node is $u$. If the algorithm asks $c$ questions to locate the target, we simply define $\mathrm{CCS}[i]=1$ for all $i>c$. Then, we can compute the average of the CCS arrays, and the result is shown in \figurename~\ref{fig:uniformIGS_Progressiveness}. The result demonstrates that our \greedy algorithm can reduce the average CSS faster than \igs on both the two datasets. On the Amazon dataset, in the worst case, \greedy and \igs need $228$ and $230$ queries respectively to locate the target node. This result is rather interesting, since our algorithm even slightly outperforms \igs for the worst-case IGS problem, although \greedy is tailored for AIGS. However, we observe that after $50$ queries, the difference between \greedy and \igs almost disappears. Hence, we only show the average CSS within the number of questions less than $50$. Similarly, we only show the CSS with the number of questions less than $100$ on the ImageNet dataset and the result exhibits a similar trend.
\begin{figure}[!tbp]
	\centering
    % \vspace{-0.1in}
	\subfloat[Amazon]{\includegraphics[width=0.3\textwidth]{figs/CSS_Tree.pdf}}\hfil
	\subfloat[ImageNet]{\includegraphics[width=0.3\textwidth]{figs/CSS_DAG.pdf}}
% 	\vspace{-0.1in}
	\caption{Progressiveness under equal probability setting.}
	\label{fig:uniformIGS_Progressiveness}
% 	\vspace{-0.2in}
\end{figure}
